# Supplementary material for: Microscopic Origin of the Valley Hall Effect in Transition Metal Dichalcogenides Revealed by Wavelength Dependent Mapping
Source: arXiv:1708.06914 ancillary file (2017-08-31)
Supplement: Supplementary file 1 [file ubrig_SI_final.pdf]

# Supporting Information

## Microscopic Origin of the Valley Hall Effect in Transition Metal Dichalcogenides Revealed by Wavelength Dependent Mapping

Nicolas Ubrig,<sup>\*,†,‡,§</sup> Sanghyun Jo,<sup>†,‡,§</sup> Marc Philippi,<sup>†,‡</sup> Davide Costanzo,<sup>†,‡</sup>  
Helmuth Berger,<sup>¶</sup> Alexey B. Kuzmenko,<sup>†</sup> and Alberto F. Morpurgo<sup>\*,†,‡</sup>

<sup>†</sup>*DQMP, Université de Genève, 24 quai Ernest Ansermet, CH-1211, Geneva, Switzerland*

<sup>‡</sup>*GAP, Université de Genève, 24 quai Ernest Ansermet, CH-1211, Geneva, Switzerland*

<sup>¶</sup>*Institut de Physique de la Matière Condensée, Ecole Polytechnique Fédérale de Lausanne,  
CH-1015, Lausanne, Switzerland*

<sup>§</sup>*Contributed equally to this work*

E-mail: [nicolas.ubrig@unige.ch](mailto:nicolas.ubrig@unige.ch); [Alberto.morpurgo@unige.ch](mailto:Alberto.morpurgo@unige.ch)

## S1 Methods

**Device fabrication.** WS<sub>2</sub> monolayer and 3R-MoS<sub>2</sub> bilayer flakes were exfoliated from bulk crystals and transferred onto Si/SiO<sub>2</sub> substrates (the silicon substrate is highly doped and could be used as gate electrode, the thickness of the oxide layer is either 90 nm or 285 nm for WS<sub>2</sub> and 285 nm for MoS<sub>2</sub> devices). The flakes were identified by looking at their optical contrast under a microscope and measuring their photoluminescence spectrum. Source and drain electrodes and Hall probes were realized by conventional nano-fabrication techniques,

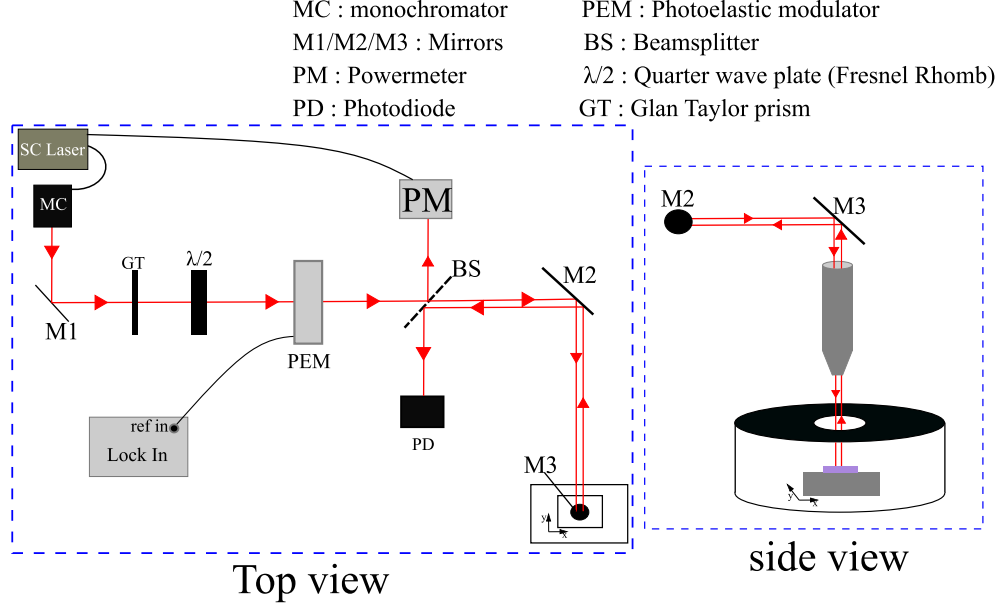

Figure S1: Schematics of the optical setup used to measure the VHE. The white supercontinuum laser is coupled to a monochromator allowing to select one specific wavelength (2nm of spectral width). The collimated laser beam passes subsequently through a Glan-Taylor prism to obtain linear polarization, then a Fresnel rhomb to control the incidence angle of the linear polarization. Modulation of circular polarized light is obtained by a photo-elastic modulator whose frequency is used as reference in lock in detecting the resulting Hall voltage. The incoming laser power is kept constant by measuring it and creating a feedback loop to the Supercontinuum laser. Reflected light on the sample is measured simultaneously with the measurement of the Hall Voltage with a photodiode to reconstruct the mapped area. The chip carrier is mounted on a x-y piezo stage with movement precision of 50nm.

based on e-beam lithography, evaporation of 50 nm Au films, and lift-off. To reduce contact resistance, the devices were annealed at 200 °C for two hours in a flow of Ar (100 sccm) and H<sub>2</sub> (10 sccm). The devices were finally mounted on a chip carrier and wire bonded. The detailed electrical characterization and transport properties of the type of monolayer WS<sub>2</sub> devices used in this study is extensively discussed in Ref. S1,S2.

**Optical measurement conditions.** All measurements were performed at T = 80 K if not stated otherwise. For the valley Hall effect measurements, the devices were illuminated using a Fianium supercontinuum laser coupled to a monochromator, providing a beam with a spectral width of 2 nm with a stabilized power (see Fig. S1). The nominal laser power to perform VHE measurements was typically set in the range 100-300 μW. The light exiting the

monochromator was coupled onto the device using an optical microscope with long working distance objectives producing a spot of approximately  $1\text{ }\mu\text{m}$  in diameter that could be focused anywhere on the TMD layer. All the measurements were done in the vacuum chamber and the chip carrier mounted inside the cryostat on a piezoelectric driven x-y stage allowing positioning precision down to 50 nm.

To support the conclusion drawn in the main text, a precise determination of the alignment between the spatial profile of the Hall voltage and the location of all contacts is of crucial importance. To this end, using a previously reported procedure,<sup>S3,S4</sup> we measure the light of the laser reflected from the sample surface simultaneously with the valley Hall data (see Fig. S1). To improve the resolution of the optical image, we use a confocal setup, in which a  $20\text{ }\mu\text{m}$  pinhole is inserted in the intermediate image plane before measuring the intensity of the reflected light with a photodiode. The reflection of the area covered with gold provides a very good contrast relative to the rest of the sample. The precise location of the electrode edges is determined by taking the position for which the reflection intensity is halfway between maximum and minimum intensity. We have verified that the procedure is reproducible and accurate. Specifically the contact edge position is determined with an experimental error estimated to be not more than 100 nm, corresponding to the smallest step size of our positioning system.

**Valley Hall effect measurements.** Linearly polarized light was produced by a Glan-Taylor prism and sent to a photoelastic modulator acting as quarter-wave plate (see Fig. S1 for the schematics of the experimental setup). The angle between the linear polarization and the fast axis of the photoelastic modulator could be adjusted by using a Fresnel rhomb with  $\lambda/2$  retardation. Circular polarization is achieved when the angle between the incident linear polarization and the fast axis of the photoelastic modulator is equal to  $45^\circ$ . The modulation frequency of the circularly and linearly (s-p) polarized light was done at 50 kHz and 100 kHz, respectively. For the circular polarization, we selected two different  $180^\circ$  shifted modulation sequences (denoted L-R and R-L in the text). The Hall voltage was detected with

a Stanford Research SR830 lock-in amplifier synchronized with the photoelastic modulator, while applying a DC source-drain bias to the device to generate the Hall Voltage (Keithley 2400).

**Photoluminescence measurement.** Photoluminescence measurements were performed in a back-scattering geometry (i.e. collecting the emitted light with the same microscope used to couple the laser beam onto the device) at an excitation wavelength of 488 nm with a laser power of 50  $\mu\text{W}$ . The light collected from the sample was sent to a Czerny-Turner monochromator and detected with a liquid Nitrogen cooled Si CCD-array.

## S2 Illustration of the effect of photodoping

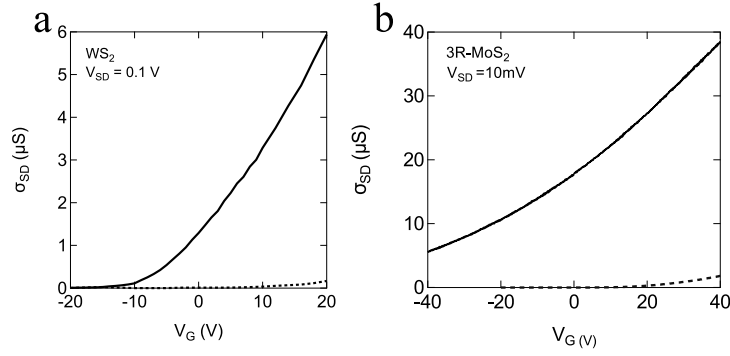

Figure S2: **a.** Representative gate voltage dependence of monolayer  $2\text{H-WS}_2$  two probe conductivity (90 nm  $\text{SiO}_2$  layer) before illumination (dashed line) and after a day of laser light exposure (solid line). The threshold voltage shifts because of persistent photodoping. After illumination, the  $V_G = 0\text{ V}$  carrier density is estimated to be  $2.5 \cdot 10^{12}\text{ V}^{-1}\text{cm}^{-2}$ . **b.** Same as **a** for our bilayer  $3\text{R-MoS}_2$  device on a substrate with an oxide layer of 300nm. Dashed and full lines represent transfer curves taken before any and after a few days of illumination respectively. The  $V_G = 0\text{ V}$  carrier density after illumination is estimated to be  $5 \cdot 10^{12}\text{ V}^{-1}\text{cm}^{-2}$ .

As mentioned in the main text, to measure the Hall voltage originating from the VHE we rely on the effect of photodoping, i.e., on the persistent conductivity that is induced in TMD layers by a prolonged exposure to light. The manifestation of photodoping on monolayer  $\text{WS}_2$  and bilayer  $3\text{R-MoS}_2$  is illustrated in Fig. S2. It is seen that for both  $\text{WS}_2$  monolayers and  $3\text{R-MoS}_2$  bilayer, as-realized devices exhibit a rather small conductivity and a positive

threshold voltage (dashed lines in Fig. S2a,b). After exposing the devices to laser light for approximately one day, the measured conductivity was systematically found to exhibit a substantial increase, accompanied by a shift in threshold voltage to negative  $V_G$  values. The conductivity induced by illumination was found to persist over time and to be sufficiently stable to perform the systematic measurements discussed in the main text.

Having measured many devices we can conclude that prolonged illumination alters both the charge density in the TMD layers (which is responsible for the threshold voltage shift) and the carrier mobility (possibly because the photo-induced charge screen defects). The investigation of the precise mechanism responsible for photo-induced change in conductivity is not known in detail and its investigation goes beyond the scope of this letter. Here we only indicate that the typical charge density values obtained by prolonged exposure to light –estimated by the measured photo-induced shift of threshold voltage– are in the range  $2.5\text{-}5 \cdot 10^{12} \text{ cm}^{-2}$ .

### S3 VHE of Bilayer 3R-MoS<sub>2</sub>

The data in Fig. 4 of the main text represent the first measurement of the VHE in non-centrosymmetric bilayer 3R-MoS<sub>2</sub> devices. Here we show additional measurements to confirm that the behavior of 3R-MoS<sub>2</sub> devices is identical in its basic aspects to that of WS<sub>2</sub> and MoS<sub>2</sub> monolayers. In particular, Fig. S3a shows the dependence of the Hall voltage on the source-drain bias,  $V_{SD}$ , measured with the laser wavelength tuned at the exciton absorption wavelength ( $\lambda = 665 \text{ nm}$ ). When changing the modulation sequence of the circular polarization state from R-L to L-R sequence, the sign of the measured Hall voltage is reversed (the R-L and L-R sequences correspond to the data represented by the blue and red curves in Fig. S3a, respectively). The data in S3a were taken with the laser spot focused at the interface with the metal contact near the Hall probes, i.e., at the position marked with the red spot

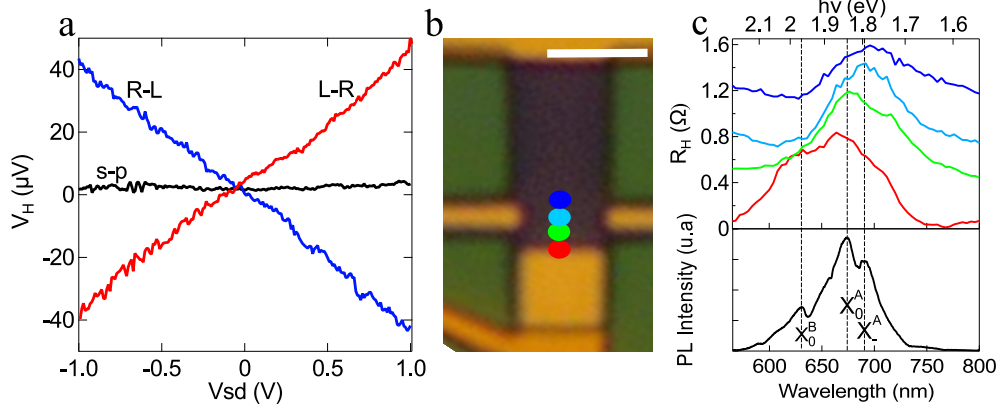

Figure S3: **a.** Hall Voltage as a function of source-drain bias measured when the laser spot is focused on the edge of the drain contact, see red dot in **b.** The wavelength is fixed at the  $X_0^A$  resonance,  $\lambda = 665 nm$ . Blue and red curve represent the R-L and L-R modulations of the polarization, while the black curve corresponds to the results of measurements done under modulation of linear polarization. The behavior is identical to the one observed in  $WS_2$  monolayers. **b.** Optical micrograph of the device. The dots indicate the laser position at which the spectra shown in **c** with lines at the corresponding colors were taken. The scale bar is  $2 \mu m$ . **c.** Top panel : Spectral dependence of the Hall Voltage measured with the laser focused on the positions shown in **b.** Bottom panel : Photoluminescence is measured on the same device, The energies of the A- and B-excitons ( $X_0^A$ ,  $X_0^B$ ) and of the trion ( $X_-^A$ ) are indicated by the dashed lines.

in the device image shown in Fig. S3b (the scale bar is  $2 \mu m$  long). If the measurements are done by modulating the light polarization between two orthogonal linearly polarized states, no Hall voltage is measured (see the black curve Fig. S3a). Similar behavior is observed for illumination at the trion absorption wavelength ( $\lambda = 690 nm$ ).

The spectral dependence of the Hall voltage measured as the position of the laser spot is varied is shown in the top panel of Fig. S3c ( $V_{SD} = -0.3V$ ; the lines of different colors are measured with the laser focused on the dot of the corresponding color in Fig. S3b). The black line in the bottom panel of Fig. S3c is the PL spectrum of the same device, irrespectively of the illumination position, in which the transitions of the A- and B-exciton ( $X_0^A$  and  $X_0^B$ ), and of the trion ( $X_-^A$ ) are clearly visible (marked with dashed vertical lines). It can be appreciated that upon moving the illumination position away from the interface

with the metal contact and towards the center of the Hall probes, the main peak in the  $R_H$  spectrum shifts from the exciton to the trion absorption wavelength. It is also worth noting that the shoulder originating from the B-exciton ( $X_0^B$ ) is more pronounced when approaching the laser close to the drain contact (see the solid red line in Fig. S3c, corresponding to the illumination position of the red point in Fig. S3b), which implies that the diffusion length of the B-exciton species is shorter than the one of the A-exciton.

## S4 Data from additional devices

In the main text we have shown maps of the VHE signal obtained from two different devices, one realized on monolayer  $WS_2$  and one on bilayer 3R- $MoS_2$ . Here we illustrate the reproducibility of the results discussed in the main text, by showing spatial maps of the VHE and the corresponding profiles as a function of the distance from the D electrode measured in three other devices, two based on  $WS_2$  monolayers (Fig. S4) and one based on 3R- $MoS_2$  bilayer (Fig. S5). In all maps, the white lines define the source and drain contact, as well as the Hall probes. The white dashed horizontal lines show the edges of the devices, while the green rectangles delimit the regions from which the horizontal profiles are calculated. The position of the middle of the Hall probes is shown by a white dashed line in the maps and a red line in the profiles. Finally, in the profiles, the yellow area correspond to the position of drain and source contact.

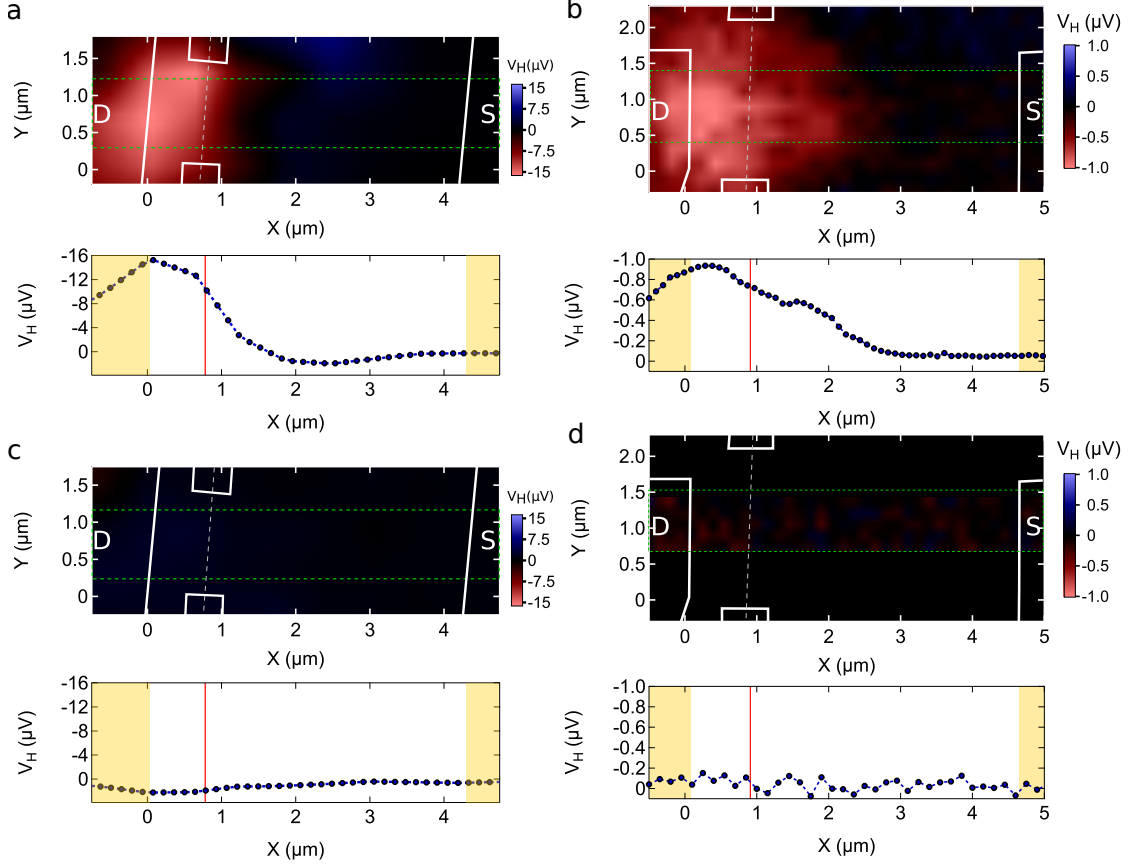

Figure S4: Maps of VHE measured on two additional  $\text{WS}_2$  monolayer devices. **a.,b.** Spatial maps (top) and extracted profiles (bottom) measured on a second and a third  $\text{WS}_2$  monolayer devices, at the exciton resonant energy ( $\lambda = 615$  nm), under circular polarization sequence. Despite the smaller amplitude, the qualitative behaviour is identical to that discussed in the main text. Panels **c** and **d** show the same measurements as the ones in panels **a** and **b**, but modulating the polarization state linearly instead of circularly. In agreement with the device shown in the main text, no significant Hall voltage is observed in this case.

Spatially resolved maps measured on two additional  $\text{WS}_2$  monolayers devices upon illumination with circular polarized light at the exciton resonance ( $\lambda = 615$  nm) are shown in Fig. S4a and Fig. S4b. As for the monolayer device discussed in the main text, the Hall voltage signal is maximum when the laser is focused at the interface with the drain contact. This is seen both in the maps and in the profiles calculated from the maps (see Fig. S4a and b bottom panels), following the same procedure discussed in Fig. 3 of the main text. Additionally, and again consistently with the behavior shown in the main text, when the measurements are done by modulating the light polarization between orthogonal linear

states no measurable signal is detected (see Figs. S4c and S4d).

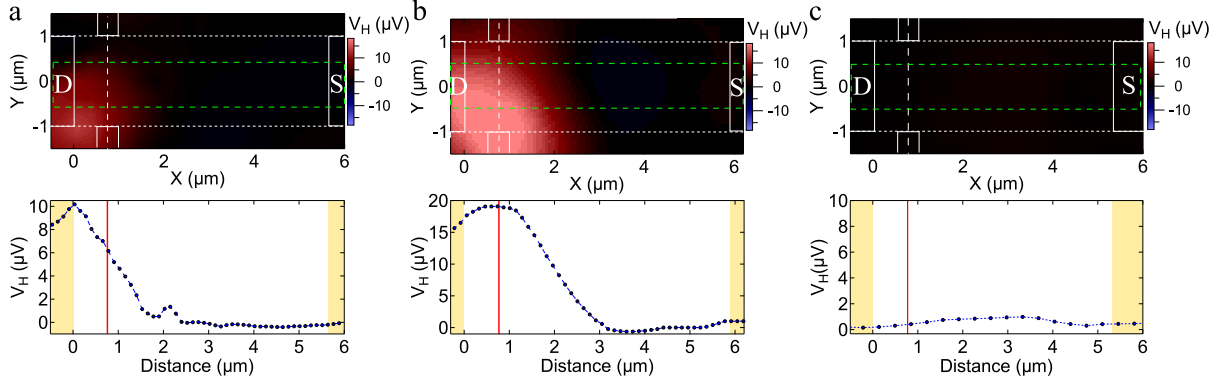

Figure S5: Measurements on a second 3R-MoS<sub>2</sub> bilayer device. **a.** Top : Spatial map of the VHE measured at the exciton resonance ( $\lambda = 665$  nm) under L-R circular polarization modulation. **b.** shows the same measurement as in **a**, but taken at the trion resonance ( $\lambda = 690$  nm). The extracted longitudinal profiles corresponding to both maps are shown in the bottom panels of **a** and **b** respectively, and allow to see the different positions of the maximum of Hall signal for the two excitations, in agreement with the behaviour presented in the main text. **c.** displays the same measurements as the ones in **a**, but with linear modulation of the polarization, displaying no Hall Voltage throughout the device.

The data for the second 3R-MoS<sub>2</sub> device are presented in Fig. S5. In particular, in the top panels of figs. S5a and S5b, we show the spatial distribution of the Hall voltage taken upon illumination at the resonant wavelength of the exciton and the trion respectively. We observe the same phenomenology as for the device discussed in the main text (see Fig. 4 of the main text). This is confirmed by the profiles of the Hall Voltage measured as the laser spot position is scanned along the channel, see bottom panels of Fig. S5a and Fig. S5b for the cases in which the laser wavelength is tuned in correspondence with the exciton and trion absorption peaks, respectively. The non-uniform distribution of the Hall voltage along the Y direction seen in Fig. S5a and S5b is most likely the consequence of a non-homogeneous contact transparency causing a non uniform density distribution near the contact. Once again, Figs. S5c show the spatial map (top) and the corresponding profile (bottom) obtained by modulating the direction of linearly (rather than circular) polarized light: no Hall voltage is observed in this case, confirming that the observation of Hall signal

requires circularly polarized light and that spurious effects due to contacts can be ruled out as argued in the main text.

## References

- [S1] Jo, S.; Ubrig, N.; Berger, H.; Kuzmenko, A. B.; Morpurgo, A. F. *Nano Letters* **2014**, *14*, 2019–2025.
- [S2] Costanzo, D.; Jo, S.; Berger, H.; Morpurgo, A. F. *Nature Nanotechnology* **2016**, *11*, 339–344.
- [S3] Reuter, C.; Frisenda, R.; Lin, D.-Y.; Ko, T.-S.; Perez de Lara, D.; Castellanos-Gomez, A. *Small Methods* **2017**, *1*, n/a–n/a.
- [S4] Mak, K. F.; McGill, K. L.; Park, J.; McEuen, P. L. *Science* **2014**, *344*, 1489–1492.
